# Supplementary material for: Low temperature magnetism of KAgF3
Source: arXiv:2212.08886 source file (2022-12-17)
Supplement: Supplementary file 1 [file supp.pdf]

# Supplementary material

## Low temperature magnetism of $KAgF_3$

John M. Wilkinson, Stephen J. Blundell, Sebastian Biesenkamp, Markus Braden, Kacper Koteras, Wojciech Grochala, Paolo Barone, José Lorenzana, Zoran Mazej, and Gašper Tavčar

Contents

S1. Purity of $KAgF_3$ samples (x-ray diffraction analysis).

S2. Exemplary Rietveld refinement results aimed to determine the purity of $KAgF_3$ samples.

S3. Computational magnetic structure prediction.
- S3.1. Magnetic superexchange calculation.
- S3.2. Spin spiral states.

S4. µSR experimental details

S5. ISIS µSR data for $T < T_{\mathrm{N1}}$

S6. Muon polarization functions
- S6.1. Muon—fluorine entangled states
- S6.2. Muon Precession

Table S1. Purity of $KAgF_3$ samples (only the crystalline phases included).

| Number | Reagents | Conditions | Composition |
|---|---|---|---|
| 1 | $KF + AgF_2 + F_2$ | 300 °C, then decomposition at 450°C, high vacuum | 99.6% $KAgF_3$<br>0.4% AgF |
| 2 | $KAg(CN)_2 + F_2$ | 300 °C, stoichiometric $F_2$ | 100.0% $KAgF_3$ |
| 3 | $KAg(CN)_2 + 5,5F_2$ | 300 °C, then decomposition at 420 °C, high vacuum | 95.8% $KAgF_3$<br>2.0% $KAgF_4$<br>2.2% $AgF_2$ |
| 4 | $AgNO_3 + KF + 1,5F_2$ | 300°C, then decomposition at 420 °C, high vacuum | 78.2% $KAgF_3$<br>21.6% $KAgF_4$<br>0.2% $AgF_2$ |
| 5 | $AgF_2 + KF$ | 300 °C, teflon, 10 days | 77.0% $KAgF_3$<br>7.2% $K_2AgF_4$<br>14.9% $AgF_2$<br>0.9% AgF |
| 6 | $1.05AgF_2 + KF$ | 300 °C, teflon, 10 days | 78.0% $KAgF_3$<br>9.1% $K_2AgF_4$<br>12.9% $AgF_2$ |
| 7 | $1.05AgF_2 + KF$ | 300 °C, teflon, 9 days | 100.0% $KAgF_3$ |
| 8 | $1.1AgF_2 + KF$ | 300 °C, teflon, 9 days | 99.0% $KAgF_3$,<br>1.0% AgF |
| 9 | $1.05AgF_2 + KF$ | 300 °C, teflon, 9 days | 100.0% $KAgF_3$ |
| 10 | $1.1AgF_2 + KF$ | 300 °C, teflon, 9 days | 99.0% $KAgF_3$,<br>1.0% AgF |
| 11 | $KF + AgF_2 + F_2$ | 300 °C, then decomposition at 450°C, high vacuum | 84.2% $KAgF_3$<br>13.7% $AgF_2$<br>2.1% $K_2AgF_4$ |

Only samples free from $AgF_2$ and $K_2AgF_4$ were used for further experiments.

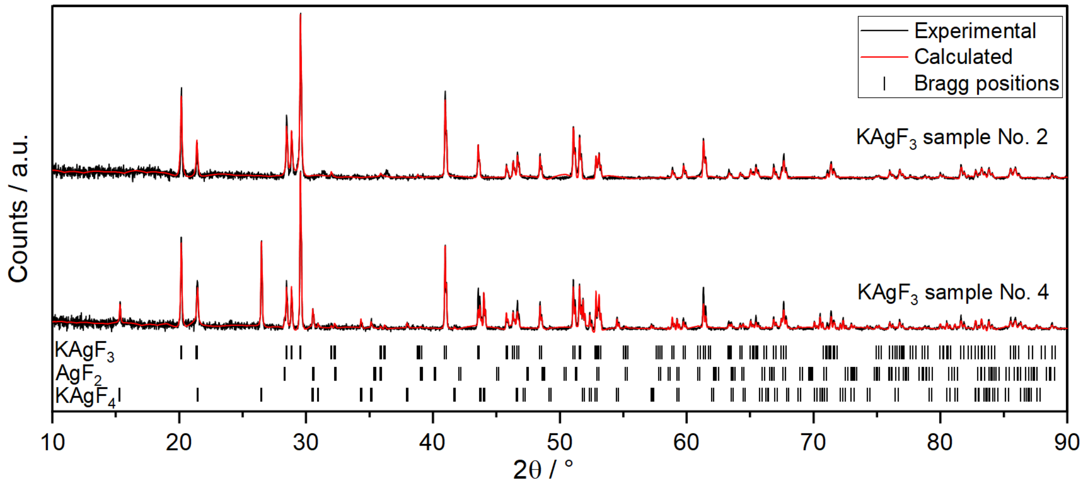


Fig S2. Exemplary Rietveld refinement results aimed to determine the purity of $KAgF_3$ samples (background subtracted).

S3. Computational magnetic structure prediction.

Based on experimental results described in the main manuscript it was possible to propose a magnetic structure of $KAgF_3$ at the low temperature. Using noncollinear, spin-orbit coupling corrected DFT+U calculations it was possible to verify the models.

Four magnetic structures were proposed, all based on well-known magnetic ground state (antiferromagnetic along ***b*** chains, ferromagnetic in $[AgF_2]$ planes on ***ac***). [1] [2] [3] Spins in these states were oriented along selected directions in crystallographic unit cell. Obtained energies of each configurations are presented below (Table S3.1).

Table S3.1 Energy of states obtained during magnetic structure determination (energy given per single Ag atom).

| Spins parallel to | [100] | [010] | **[001]** | [101] |
|---|---|---|---|---|
| Relative energy / meV | 0.708 | 0.078 | **0.000** | 0.452 |
| Relative energy / K | 8.21 | 0.91 | **0.00** | 5.24 |

In agreement with neutron diffraction and μSR data, lowest energy magnetic structure is one, where spins are parallel to crystallographic ***c*** axis. Structure with magnetic moment parallel to ***b*** axis has only slightly higher energy. Interesting is the fact, that orientation of magnetic moment parallel to ***a*** axis shows significant increase of energy. The difference can be attributed to orthorhombic distortion and spin-orbit coupling that is stabilizing the [001] solution. Unpaired electron, which is providing magnetic moment, resides on Ag $d_{x^2-y^2}$ orbital which has alternating orientation at neighbouring Ag sites due to cooperative Jahn-Teller effect. [3]

S3.1. Magnetic superexchange calculation

Reported magnetic susceptibility measurements point to two phase transitions of unknown origin between the ground state $KAgF_3$ (*Pnma*) structure and high temperature disordered *Pcma* polymorph. The abovementioned neutron diffraction results, and previously reported synchrotron data together mean, that possible phase transitions are not structural. Based on the fact, that $KAgF_3$ is a strongly correlated material with an extraordinary magnetic properties, a theoretical study was conducted in order to predict possible intermediate phases.

Previously reported calculations of magnetic superexchange constants $J$ include only two, nearest neighbour interactions ($J_{1D}$ and $J_{ac}$ on Figure S3.1.1). One of the factors that can lead to higher energy magnetic orders is magnetic frustration, where a pair of spins experience opposing exchange forces. In order to verify that possibility, two additional next nearest neighbour interactions were taken into account ($J_a$ and $J_c$ on Figure S3.1.2).

Calculation of all four constants simultaneously proved to be difficult and yielded very excitation selection dependent results. Probable cause of that is the fact, that $J_{ac}$, $J_a$ and $J_c$ constant differ in orders of magnitude from $J_{1D}$ and errors in determination of the last one affect precise determination of the three in-plane constants. Because of that, two-step process was introduced in which $J_{1D}$ is calculated separately from other three. $J_{1D}$ was determined to be equal to 172.3 meV using calculated energy of antiferromagnetic ground state and ferromagnetic excited state. This value is significantly bigger than the previously reported values, but such a discrepancy is expected while using simplified model. The aim of this calculations was to determine precisely intralayer constant and this result is not affecting them.

Excited states selected for calculation of three in-plane constants were chosen specifically to not break an antiferromagnetic order along crystallographic ***b*** (Figure S3.1.1 and Table S3.1.3). Values of superexchange constants were calculated using least squares method, as the system of eight equations and four variables is overdetermined. Determined value of $J_{ac}$ is equal to -3.8 meV, being very close

to previously reported values (-5.8 meV [3] and -2.6 meV [1]). The values of $J_a$ and $J_c$ are unsurprisingly very small, reaching -0.4 and -0.5 meV correspondingly. The difference between these two comes from orthorhombicity of the unit cell. Crystallographic ***c*** vector is smaller than ***a*** (6.0581(8) *vs* 6.3815(9) Å), thus shortening Ag-F bond length and increasing *d* orbital overlap increase superexchange.
All three constants are ferromagnetic, meaning that in the ground state, where [$AgF_2$] planes in $KAgF_3$ are ordered ferromagnetically, there is no magnetic frustration.

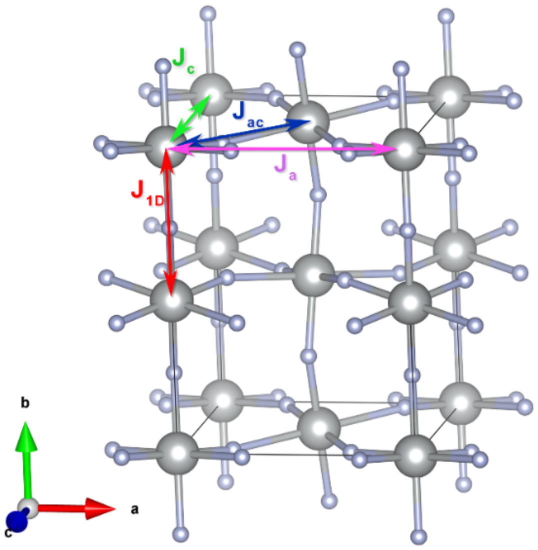


Fig S3.1.1 Depiction of considered types of superexchange pathways in $KAgF_3$ calculations (Ag – grey, K – omitted, F – light blue).

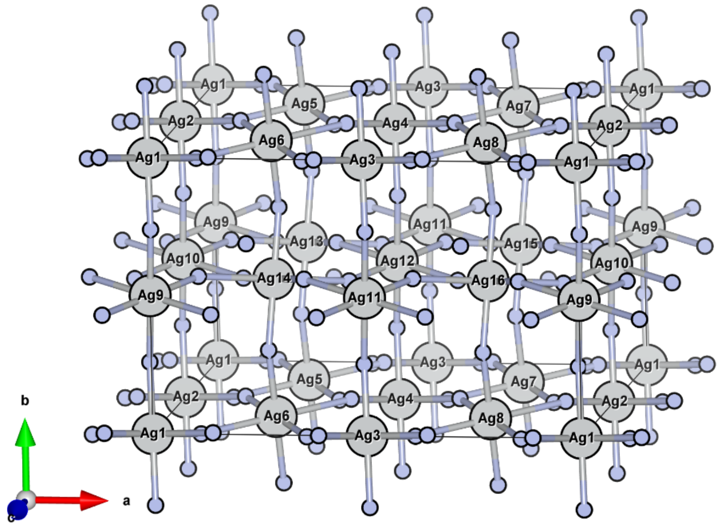


Fig.S3.1.2 $KAgF_3$ supercell used in extended magnetic superexchange calculation (some atoms omitted for clarity; Ag – grey, F – light blue).

Table S3.1.3. Different magnetic states used in calculation of superexchange constants (Ag1-Ag16 symbolize different silver atoms in the supercell; A1-P8 denote different excitation states; superexchange constants were derived as a solution of set of equation resulting from Heisenberg model; total energy values are given per full supercell).

| | A1 | F1 | P1 | P2 | P3 | P4 | P5 | P6 | P7 | P8 |
|---|---|---|---|---|---|---|---|---|---|---|
| Ag1 | + | + | + | + | − | − | + | − | − | − |
| Ag2 | + | + | + | + | + | + | + | + | + | + |
| Ag3 | + | + | + | + | − | + | + | − | + | − |
| Ag4 | + | + | − | − | + | − | + | − | + | − |
| Ag5 | + | + | + | + | + | + | − | + | + | + |
| Ag6 | + | + | + | + | − | − | + | + | − | − |
| Ag7 | + | + | + | − | + | − | − | + | + | + |
| Ag8 | + | + | + | − | + | + | + | + | + | + |
| Ag9 | − | + | − | − | + | + | − | + | + | + |
| Ag10 | − | + | − | − | − | − | − | − | − | − |
| Ag11 | − | + | − | − | + | − | − | + | − | + |
| Ag12 | − | + | + | + | − | + | − | + | − | + |
| Ag13 | − | + | − | − | − | − | + | − | − | − |
| Ag14 | − | + | − | − | + | + | − | − | + | + |
| Ag15 | − | + | − | + | − | + | + | − | − | − |
| Ag16 | − | + | − | + | − | − | − | − | − | − |

Simplified model:

$E_{A1} = E_0 + 4J_{1D}$
$E_{F1} = E_0 - 4J_{1D}$

Extended model:

$E_{P1} = E_0 + 4J_{ac} + 2J_a + 2J_c$
$E_{P2} = E_0 - 2J_a + 2J_c$
$E_{P3} = E_0 + 2J_a - 2J_c$
$E_{P4} = E_0 - 4J_a - 4J_c$
$E_{P5} = E_0 + 4J_a$
$E_{P6} = E_0 - 4J_{ac} + 2J_a + 2J_c$
$E_{P7} = E_0 + 2J_{ac}$
$E_{P8} = E_0 - 2J_{ac}$

$$J_{1D} = 2(E_{F1} - E_{A1}) = 172.3 \text{ meV}$$
$$J_{ac} = -3.8 \text{ meV}, \quad J_a = -0.4 \text{ meV}, \quad J_a = -0.5 \text{ meV}$$

S3.1.2. Spin spiral states.

As a proposition of intermediate magnetic phase of $KAgF_3$, for the temperature range from 30 K to 65 K, different types of spin spiral were proposed. Long range order in the [$AgF_2$] planes was hinted by a weak peak in neutron pattern, that has gained intensity at *ca.* 40 K. As it was mentioned in the main paper, it can be indexed as (1/3, 0, 1/3).

In order to accommodate magnetic configurations with longer ordering vectors than the unit cell, the 3√2×1×√2 supercell was used (Figure S3.1.2.1). The notation, used in this section to describe spiral magnetic configurations, is however consistent with unit cell frame of reference.

First, two basic types of spiral were selected with ordering vectors equal to (1, 0, 1) for the AF spiral and (1/3, 0, 1/3) for the F spiral. In other words, magnetic moments on two adjacent Ag centres, along the magnetic ordering vector make 120° in the AF spiral setting and 60° in the F spiral configuration. Notation of these spirals stems from the fact, that both can be viewed as a distortion from antiferromagnetically (AF) and ferromagnetically (F) ordered [$AgF_2$] planes in $KAgF_3$. Selected spirals are presented below in a supercell (Figure S3.1.2.3).

First, the calculation without inclusion of spin-orbit coupling was conducted. Magnetic moments were then noncollinear, but it was not determined how were the spirals placed. Chirality in this approach was also not accounted for. Obtained relative energies are presented in the Table S3.1.2.2. In agreement with prediction, the F spiral has lower energy than the AF spiral, due to the fact, that the ground state is ordered ferromagnetically in the [$AgF_2$] planes. Thermal equivalent of the relative

energy of the F spiral is equal to 2.82 K and the AF spiral is a couple times higher, reaching 14.47 K. Of course, relative energy difference obtained with DFT+U calculations rarely is an accurate prediction of phase transition temperature, but the latter value is of the right order of magnitude.
Main result here is the fact, that both spirals were stable solutions in a DFT+U framework, and that they are qualitatively a higher energy magnetic configuration.

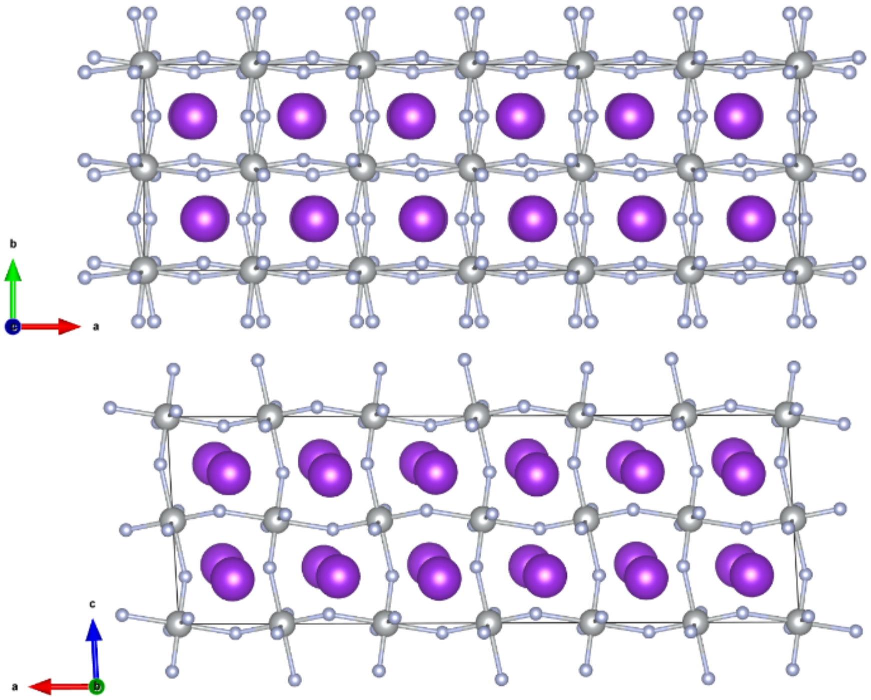


Fig S3.1.2.1. $KAgF_3$ 3√2´1´√2 supercell used in noncollinear calculations (Ag – grey, K – purple, F – light blue).

Table S3.1.2.2. Relative energies of spin spiral state calculated without spin-orbit coupling (energy given per single Ag atom, related to energy of a ground state calculated without spin-orbit coupling).

| Magnetic configuration | AF spiral (120° step) | F spiral (60° step) |
|---|---|---|
| Relative energy / meV | 1.247 | 0.243 |
| Relative energy / K | 14.47 | 2.82 |

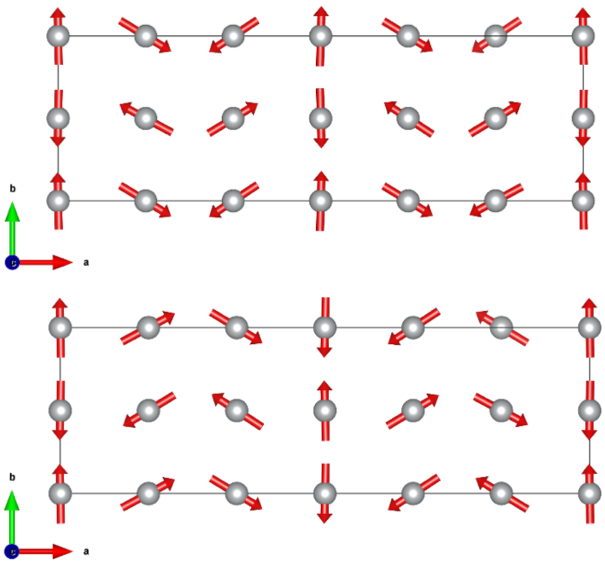


Fig S3.1.2.3. Two selected spin spiral configurations in a $KAgF_3$. Right hand AF spiral places on $(10\bar{1})$) (top) and Right hand F spiral placed on $(10\bar{1})$ (bottom). (K and F atoms omitted for clarity, magnetic moments shown as red arrows)

In the next step, calculations including spin-orbit coupling were conducted. In these types of calculation not only the relative orientation between adjacent spins affects the energy, but their relative orientation with the lattice. Inclusion of spin orbit coupling allows for analysis of chirality of spin spirals as well. Energies of four different spin spiral orientations for every spin spiral were calculated, together with their right-hand and left-hand types (Table S.3.1.2.4).
Similar tendencies as in calculations without spin-orbit coupling were found. Generally, the F spirals had lower energy, than the AF spiral. Lowest energy spiral always was the one placed on (100) plane, (note, in the antiferromagnetic ground state, magnetic moments are parallel to the [001] direction). Orientation of the spiral at (100) plane provides closest solution to the ground state then. Other orientations were chosen such that at least one provides a proper spiral (where the ordering vector is normal to the plane that the spiral is placed on), that is (101) setting. Other two orientations ($(10\bar{1})$ and (010)) were chosen in such a way, that they include the ordering vector on the same plane that the spiral was placed on. The handedness of the spin spirals does not affect their energy in any significant way as the differences in relative energy were probably stemming from numerical errors.

Table S.3.1.2.4. Relative energies of spin spiral state calculated with spin-orbit coupling (energy given per single Ag atom; related to energy of a ground state calculated with spin-orbit coupling; crystallographic planes given for the unit cell frame of reference).

| | Spin spiral orientation | Right-hand / meV (/ K) | Left-hand / meV (/ K) |
|---|---|---|---|
| AF spiral (120° step) | $(10\bar{1})$ | 1.362 (15.81) | 1.378 (15.99) |
| | (101) | 1.346 (15.62) | 1.347 (15.62) |
| | (010) | 1.513 (17.55) | 1.501 (17.42) |
| | (100) | 1.157 (13.43) | 1.155 (13.40) |
| F spiral (60° step) | $(10\bar{1})$ | 0.370 (4.29) | 0.376 (4.36) |
| | (101) | 0.349 (4.05) | 0.365 (4.24) |
| | (010) | 0.509 (5.91) | 0.533 (6.19) |
| | (100) | 0.188 (2.18) | 0.164 (1.90) |

These results were confirmed using calculation based on modified model. Generally, assuming collinear spin orientation, the Heisenberg Hamiltonian is equal to

$$H = E_0 + 0.5\sum_{i,j} J_{ij} s_i s_j \,,$$

where $s_i$ and $s_j$ are magnetic moments on adjacent paramagnetic sites and their values can be positive or negative. In the case of noncollinear magnetism, magnetic moments can be expressed as vectors, and Hamiltonian then takes the form of

$$H = E_0 + 0.5\sum_{i,j} J_{ij}\mathbf{S}_i\mathbf{S}_j = E_0 + 0.5\sum_{i,j} J_{ij} S_i S_j \cos\theta_{ij}\,,$$

where $\mathbf{S}_i$ and $\mathbf{S}_j$ are vector magnetic moments, $S_i$ and $S_j$ are magnitudes of magnetic moments and $\theta_{ij}$ is the angle between two spins on adjacent sites that are coupled with $J_{ij}$ constant. Collinear solution is easily derived from that model, as possible angles are 0° and 180° leading to 1 and –1 value of $\theta_{ij}$.

Application of superexchange constants determined above to Heisenberg Hamiltonian allowed for model prediction of noncollinear spin spirals (Table S.3.1.2.5). Energies obtained that way show similar tendencies as these calculated in noncollinear DFT+U framework. Relative energies derived from the model are however higher. Collinear model does not include anisotropic interactions, so it is not unexpected.

Table S.3.1.2.5. Relative energies of spin spiral state calculated from Heisenberg model (energy given per single Ag atom, related to the A1 ground state).

| Magnetic configuration | AF spiral (120° step) | F spiral (60° step) |
|---|---|---|
| Relative energy / meV | 1.751 | 0.584 |
| Relative energy / K | 20.32 | 6.78 |

S.4 µSR experimental details

In the muon experiments, a beam of spin-polarized muons were incident on the sample which was placed in a copper sample holder, and the number of positrons detected in both the forwards and backwards detectors, $N_\mathrm{F}(t)$ and $N_\mathrm{B}(t)$ respectively, was measured [1] [2]. The muon asymmetry was calculated as

$$A(t) = \frac{N_\mathrm{B}(t) - \alpha N_\mathrm{F}(t)}{N_\mathrm{B}(t) + \alpha N_\mathrm{F}(t)}$$

where the parameter $\alpha$ takes into account systematic differences between the readings of both sets of detectors. Our experiments were performed using the MuSR spectrometer at the ISIS Facility, Rutherford Appleton Laboratory, UK and the GPS spectrometer at PSI, Villigen, Switzerland. The Earth's magnetic field was compensated to better than 50 µT using active field compensation. The mean muon lifetime is 2.2 µs, but reliable data can be obtained out to at least ten times this value at ISIS if collected for several hours.

## S.5 ISIS μSR data for $T < T_{\mathrm{N1}}$

The μSR data taken at ISIS for selected temperatures showing the onset of magnetic order are displayed in Figure S5.1. Due to the superior statistics of this dataset, it is possible to measure the muon asymmetry over a much longer timescale than the PSI data, although it is not possible to resolve the oscillations at the shorter timescales (as shown in the inset). These data show that clear F–μ–F oscillations start to appear at 30 K, and are very pronounced at about 40 K. The presence of these oscillations is indicative of a lack of magnetic order, as the dipole-dipole coupling between the muon and fluorine is much smaller than the Zeeman interaction of the muon in its local magnetic field.

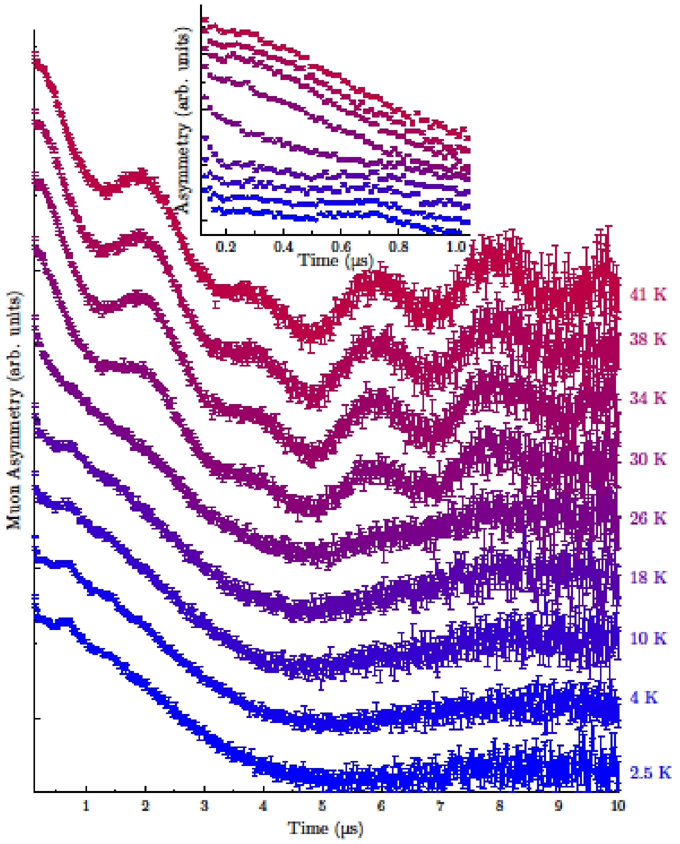


Figure S5.1: μSR data taken with the MuSR spectrometer at ISIS. The oscillations observed above 30 K are due to the muon entering into a F–μ–F state, due to the entanglement between the muon and the nearest fluorine nuclei. Inset: the data in the main frame at short times, showing the onset of magnetic order in the sample, which is resolved better in the PSI data plotted in the main text.

## S6 Muon polarization functions

### S6.1 Muon—fluorine entangled states

The aim of the muon experiment is to obtain the time dependence of the muon polarization $P_{\mu}^{\hat{\boldsymbol{n}}}(t)$, where $\hat{n}$ denotes the direction of the initial muon polarization. This can be simulated using

$$P_{\mu}^{\hat{\boldsymbol{n}}}(t) = \mathrm{Tr}[\rho(t)\boldsymbol{\sigma}_{\mu} \cdot \hat{\boldsymbol{n}}]$$

where ρ(t) is the density matrix of the muon and its environment, and $\boldsymbol{\sigma}_{\mu}$ is the Pauli spin operator of the muon, projected on the initial muon polarization direction $\hat{\boldsymbol{n}}$ (due to the geometry of the instrument). When a muon is implanted in a sample, it interacts with the surrounding nuclear spins by means of the dipole-dipole Hamiltonian $\mathcal{H}$, given by

$$\mathcal{H} = \sum_{i>j} \frac{\mu_0 \gamma_i \gamma_j}{4\pi\hbar |\boldsymbol{r}_{ij}|^3} [\boldsymbol{s}_i \cdot \boldsymbol{s}_j - 3(\boldsymbol{s}_i \cdot \hat{\boldsymbol{r}}_{ij})(\boldsymbol{s}_j \cdot \hat{\boldsymbol{r}}_{ij})] + \sum_i \boldsymbol{\mu}_i \cdot \boldsymbol{B}_i,$$

where $\boldsymbol{r}_{ij}$ is the vector linking spins $i$ and $j$, and $\boldsymbol{B}_i$ is the magnetic field at the site of the nuclear moment $\boldsymbol{B}_i$, and all other symbols have their usual meanings. For the case of a muon interacting with

spin-$\frac{1}{2}$ fluorine ($^{19}$F) nuclei ($\gamma_{\mathrm{F}} = 2\pi \times 40.061$ MHz T$^{-1}$) in zero field, the muon's polarization evolves in an observable pattern of beats (the frequencies of which provide information of the surrounding nuclei, due to the $\boldsymbol{r}_{ij}$ dependence of the Hamiltonian), with a relaxation which is due to the system decohering with the environment of further nearest-neighbours, which have a weaker, but non-negligible coupling to the muon.

Including all the nuclei in the sample directly in this Hamiltonian is not possible since the dimension of $\mathcal{H}$ grows exponentially with the number of spins included. Therefore, following [3] and [4] we cut off our Hilbert space to include enough nearest neighbours to describe the main features of the µSR asymmetry, and then rescale the coupling to the k ions most distant to the muon using a parameter $\zeta_k$ which is chosen so that the second moment of our reduced system matches that of the infinite system. The variance of the field distribution at the muon site caused by $M$ spins is $\left(\frac{\sigma M}{\gamma_\mu}\right)^2 = \frac{2}{3}\left(\frac{\mu_0}{4\pi}\right)^2 \hbar^2 \sum_{j=1}^{M} \frac{\gamma_j^2 I_j(I_j+1)}{r_j^6}$, where $r_j$ is the distance from the muon to the $j$th nucleus with spin $I_j$ and gyromagnetic ratio $\gamma_j$, $\gamma_\mu$($= 2\pi \times 135.5$ MHz T$^{-1}$) is the muon gyromagnetic ratio, and the sum converges as $M \to \infty$. We then calculate $\zeta_k$ from

$$\sigma_\mu^2 = \sigma_{\mathrm{nn}}^2 + \frac{2}{3}\left(\frac{\mu_0}{4\pi}\right)^2 \hbar^2 \gamma_\mu^2 \sum_{j\in k} \frac{\gamma_j^2 I_j\left(I_j+1\right)}{\left(\zeta_k r_j\right)^6},$$

and then evaluate our exact calculation of the muon polarization to the restricted set of spins comprising the muon, the nearest-neighbours, and the set of $k$ ions (with the distance between the ion and the muon rescaled by $\zeta_k$.).

S6.2 Muon Precession

In samples which are magnetically ordered, the dipolar interactions in the muon's Hamiltonian tend to be much smaller than the Zeeman term ($\propto \boldsymbol{\mu} \cdot \boldsymbol{B}$), and therefore can usually be neglected. It is easy to show that the muon polarization in this case is simply $P_\mu(t) = cos(B_\mu \gamma_\mu t)$ for a magnetic field in a perpendicular direction to the initial muon polarization. Because of inhomogeneities in the magnetic field at the muon site, the oscillations in the muon polarization tend to decay in a fashion which is modelled well by an exponential decay function of the form $e^{-\lambda t}$.

**References**


[1] D. M. Z. Kurzydłowski, Z. Jagličić, Y. Filinchuk and W. Grochala, "Structural transition and unusually strong antiferromagnetic superexchange coupling in perovskite KAgF3," *Chemical Communications,* vol. 49, no. 57, pp. 6262-6264, 2013.

[2] D. Kurzydłowski and W. Grochala, "Large exchange anisotropy in quasi-one-dimensional spin-1/2 fluoride antiferromagnets with a d(z2)1 ground state," *Physical Review B,* vol. 96, no. 15, p. 155140, 2017.

[3] X. Zhang, G. Zhang, T. Jia, Y. Guo, Z. Zeng and H. Q. Lin, "KAgF3: Quasi-one-dimensional magnetism in three-dimensional magnetic ion sublattice," *Physics Letters A,* vol. 375, no. 24, pp. 2456-2459, 2011.

[4] S. F. J. Cox, "Implanted muon studies in condensed matter science," *J. Phys. C: Solid State Phys.,* vol. 20, p. 3187, 1987.

[5] S. J. Blundell, R. De Renzi, T. Lancaster and F. L. Pratt, Muon Spectroscopy: An Introduction, Oxford: Oxford University Press, 2022.

[6] J. M. Wilkinson and S. J. Blundell, “Information and Decoherence in a Muon--Fluorine Coupled System,” *Phys. Rev. Lett.,* vol. 125, p. 087201, 2020.

[7] J. M. Wilkinson, F. L. Pratt, T. Lancaster, P. J. Baker and S. J. Blundell, “Muon sites in PbF2 and YF3: Decohering environments and role of anion Frenkel defects,” *Phys. Rev. B,* vol. 104, p. L220409, 2021.
